# Supplementary material for: Microalgae scatter off solid surfaces by hydrodynamic and contact forces
Source: arXiv:1511.00888 source file (2015-11-03)
Supplement: Supplementary file 1 [file SupplementaryMaterial_2.pdf]

# Microalgae scatter off solid surfaces by hydrodynamic and contact forces
# Supplementary Material

Matteo Contino, Enkeleida Lushi, Idan Tuval, Vasily Kantsler and Marco Polin

## SUPPLEMENTARY MOVIES

- "WT_contact_1,2,3" are examples of contact deterministic scattering by CC125 cells;
- "WT_random_1,2" are examples of random scattering by CC125 cells;
- "SHF_contact" and "SHF_random" are examples of deterministic contact and random scattering by SHF1 mutants;
- "Sim_1" and "Sim_2" are simulation movies demonstrating the escape of the model swimmer from trapping due to cell spinning.

## DETERMINISTIC SCATTERING

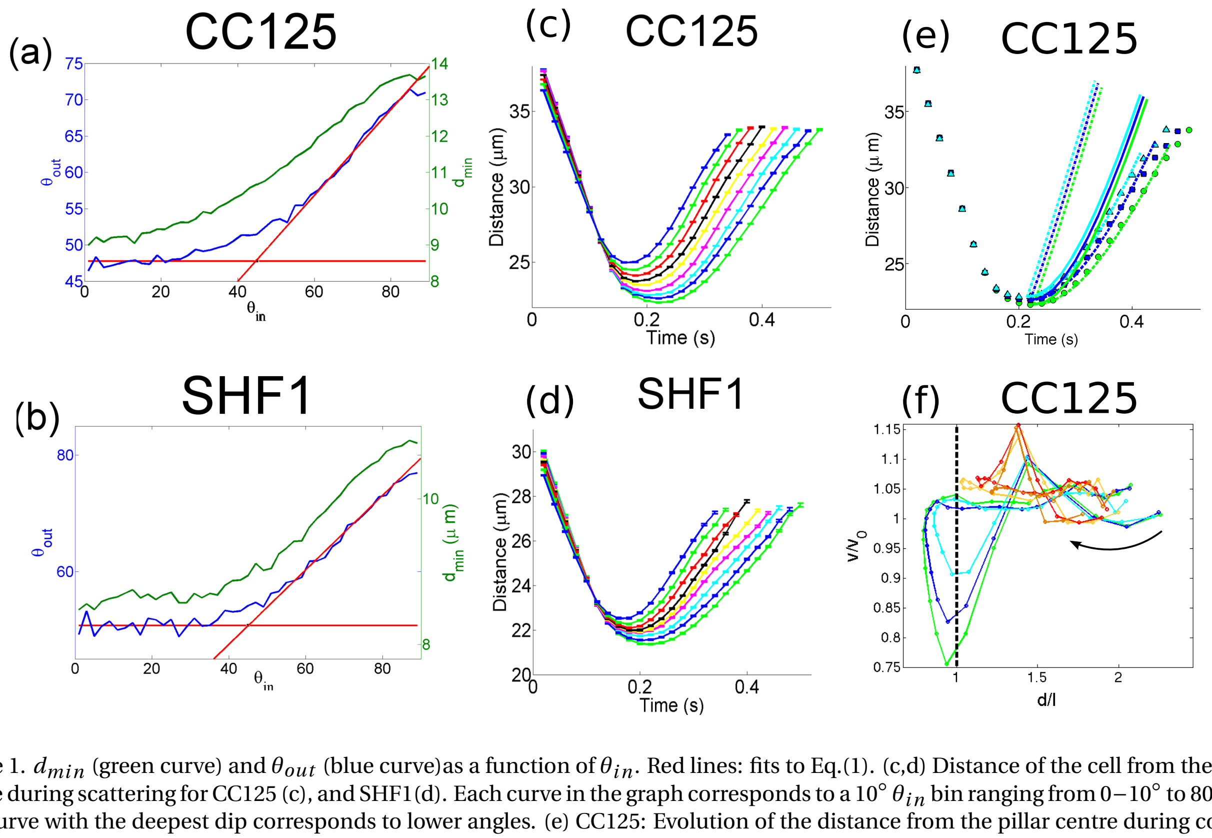


Figure 1. $d_{min}$ (green curve) and $\theta_{out}$ (blue curve)as a function of $\theta_{in}$. Red lines: fits to Eq.(1). (c,d) Distance of the cell from the pillar centre during scattering for CC125 (c), and SHF1(d). Each curve in the graph corresponds to a $10^\circ$ $\theta_{in}$ bin ranging from $0-10^\circ$ to $80-90^\circ$. The curve with the deepest dip corresponds to lower angles. (e) CC125: Evolution of the distance from the pillar centre during contact interaction, for $\theta_{\text{in}}$ in $[0^\circ, 10^\circ]$ (◯); $[10^\circ, 20^\circ]$ (□); $[20^\circ, 30^\circ]$ (△). Lines are best fits to: straight swimming after recovery at an exit angle $\theta_{\text{out}} = 48^\circ$ (dot-dashed lines); straight swimming after recovery with a trajectory tangent to the pillar surface (solid lines); swimming on a circular trajectory off-centred from the pillar (dashed lines. Radii of curvature $\rho_{exp} = (36.5\,\mu\text{m}, 45.6\,\mu\text{m}, 57\,\mu\text{m})$ for green, blue, and cyan data respectively). All fits are based on the observed swimming velocity of $v_0 = 106.4\,\mu\text{m/s}$. (f) Scattering trajectories in the $(v/v_0, d/\ell)$ plane. $\ell$: average flagellar length. Different $\theta_{in}$ are colour coded as in the main paper. The arrow indicates the beginning of the trajectory. Dashed line highlights $d = \ell$.

## LARGER PILLARS

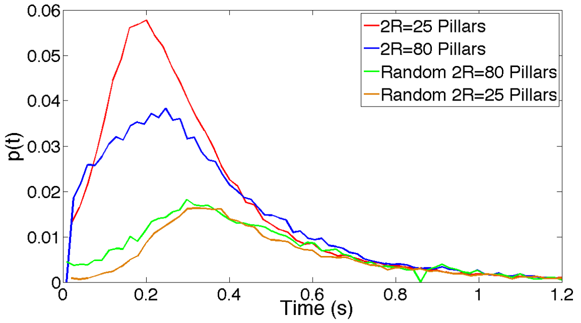


Figure 2. Comparison between the distributions of scattering events' duration for 40 $\mu$m-radius and 12.5 $\mu$m-radius pillars. For the larger pillars, the interpillar distance was 180 $\mu$m and $\sim$ 20k events were recorded. Strain used: CC125.

## RANDOM SCATTERING

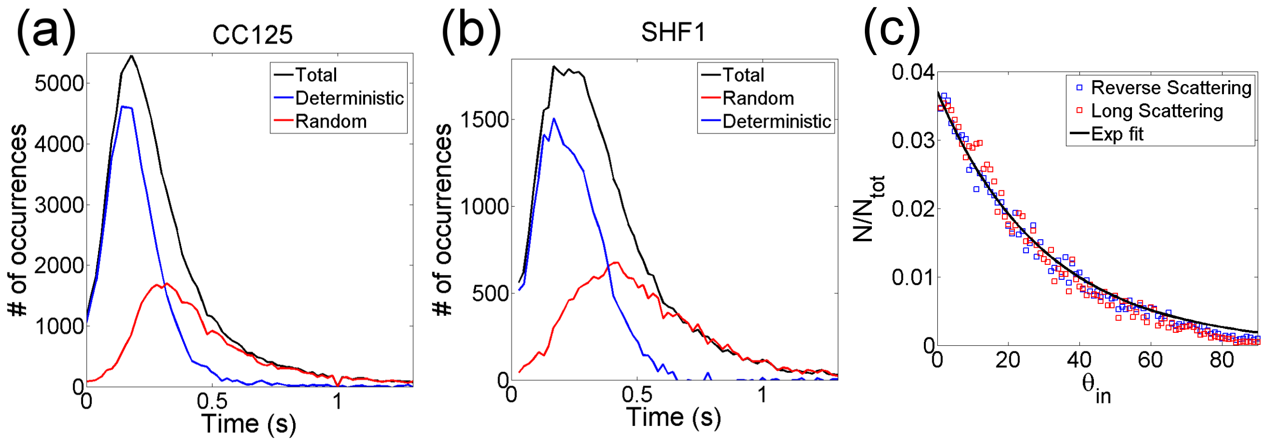


Figure 3. Distribution of scattering duration for CC125 (a) and SHF1 (b), irrespective of $\theta_{\rm in}$. (c) Distribution of $\theta_{\rm in}$ for scattering events with negative $\theta_{\rm out}$ (blue squares) and with duration longer than 0.75 s (red squares) for CC125. Both distribution are well fitted by the curve $p(\theta_{\rm in}) = 0.038 * \exp(-\theta_{\rm in}/\theta^*)$, $\theta^* = 50°$ (black line) which also well represents the distribution for random scattering.

Direct collision with the pillar can cause *Chlamydomonas* to perform "random" scattering: it aligns along the short dimension of the sample cell; then alternates periods of clockwise and counter-clockwise swimming around the pillar; and eventually leaves the scattering corona with an equal probability of having positive or negative $\theta_{\rm out}$ (see supplementary movies: Random1, Random2, Random3, ShortRandom1, ShortRandom2). During "deterministic" scattering, instead, $\theta_{\rm in}$ and $\theta_{\rm out}$ have the same sign, and the cell moves exclusively along the focal plane of the objective. Negative scatterings, i.e. those with opposite signs for $\theta_{\rm in}$ and $\theta_{\rm out}$, are certainly "random", and are readily recognised among the thousands of scatterings recorded at low-magnification. The red lines in Fig. 3(a,b) show the distribution of the duration of negative scattering events for each of the two strains used, **multiplied by 2**. We use this to approximate the curve that would be obtained from all of the random scatterings. The agreement between the tails of the red and black curves in Fig. 3(a,b) supports this assumption, since long-lasting scatterings are certainly exclusively random. This was further tested by selecting all the events lasting longer than 0.75 s, and comparing their behaviour with that of all negative scattering events. We find consistently good agreement between the two, as shown e.g. in Fig. 3(c). The distributions in 3(a,b) are then used to set thresholds in the scattering duration allowing us to either retain most of the deterministic scattering events and discard most of the random ones (events lasting less than 0.32 s) or *vice versa* (events lasting longer than 0.75 s). The scattering angles' distributions in Figs. 1,4 of the main text do not change appreciably if different thresholds are selected, as long as the new thresholds are lower/higher than those we report above, for deterministic/random events respectively.

## SIMULATIONS

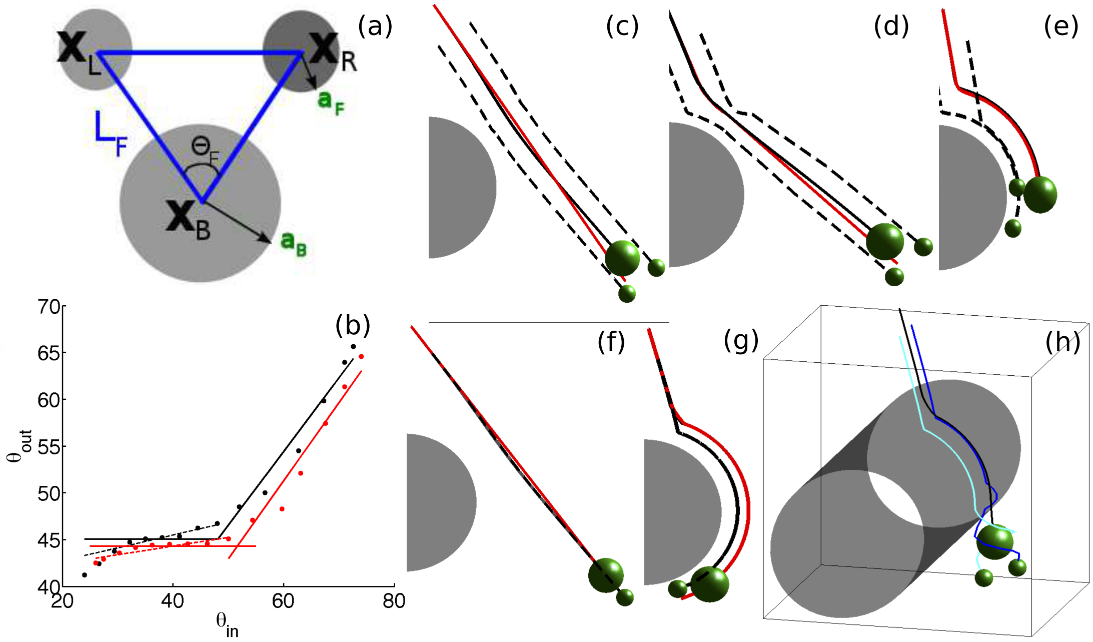


Figure 4. (a) Schematics of the simulation model; (b) Scattering angle $\theta_{\text{out}}(\theta_{\text{in}})$ for simulations a swimmer in the configuration perpendicular to the pillar surface, with $L_F = 2\,a_B$ and $L_F = 1.8\,a_B$ (black and red circles respectively). Solid lines are fits to Eq. (1) in the main text, where the fit values can be found in Table I. The dashed lines are linear fits for the simulated points in the range $\theta_{\text{in}} \in [25°, 45°]$, with slopes $m = 0.137$ (black dashed line) and $m = 0.1$ (red dashed line). (c-e) Non-rotating swimmer with flagella configuration perpendicular to the surface. Examples of (c) hydrodynamic regime; (d) scattering regime; (e) trapping regime. (f,g) Non-rotating swimmer with flagella configuration parallel to the surface. Examples of (f) hydrodynamic regime; (g) trapping regime. This configuration does not display a scattering regime. Red lines are trajectories where hydrodynamics has been switched off. (h) Rotation-mediated escape: a swimmer with configuration tangential to the pillar surface is trapped and orbits around the obstacle, but it can escape when the rotation about the main axis is switched on.

We consider a minimal "puller" swimmer model consisting of three Stokeslet beads connected by springs (Fig. 4(a)) with constant propulsive forces concentrated on the two flagella beads of radius half the body-bead. Zero net force determines the coupled dynamics of the beads $B, L, R$ (denoting the body, left and right flagellum beads respectively) to be

$$\frac{d\mathbf{x}_k}{dt} = \frac{1}{\xi_k}\left[\delta_{k,(L,R)}\mathbf{f}^f_k + \mathbf{f}^c_k + \mathbf{f}^x_k\right] + \sum_{j=(B,L,R)} G_{a_j}(\mathbf{x}_k, \mathbf{x}_j)\left[(1-\delta_{k,j})\mathbf{f}^c_j + \mathbf{f}^x_j\right] + \sum_{j=(B,L,R)} \tilde{G}_{a_j}(\mathbf{x}_k, \mathbf{x}_j)\left(\mathbf{f}^c_j + \mathbf{f}^x_j\right)$$

for $k = (B, L, R)$. Here $\xi_k = 6\pi a_k$ are the Stokes drag coefficients and $a_B = 1/3$, $a_L = a_R := a_F = 1/6$ are the bead radii. The propulsive forces $\mathbf{f}^f_L$ and $\mathbf{f}^f_R$ act only on the two flagella beads $L$ and $R$. The connector spring forces $\mathbf{f}^c$ follow a finitely extensible nonlinear elastic (FENE) spring model. The repulsive steric forces $\mathbf{f}^x_k$ are calculated with the Lennard-Jones potential activated at $2^{1/6}a \approx 1.12a$ distance away from a bead's centre.

$$G_a(\mathbf{x}_k, \mathbf{x}_j) = \frac{1}{8\pi}\left[\frac{r^2 + 2a^2}{(r^2+a^2)^{3/2}}\mathbf{I} + \frac{(\mathbf{x}_k - \mathbf{x}_j)(\mathbf{x}_k - \mathbf{x}_j)^T}{(r^2+a^2)^{3/2}}\right]$$

with $r = ||\mathbf{x}_k - \mathbf{x}_j||$, is a regularised 3D Stokeslet where the regularisation parameter $a$ is the radius of the bead. Near a no-slip wall, the method of Stokeslet images, here denoted by $\tilde{G}_a$, are employed to calculate the fluid flow at each bead's position. The wall in this case is a cylindrical pillar, so the regularised image Stokeslet system is modified accordingly for a cylindrical surface where the no-slip condition holds. The following parameters are used to approximate the experiments: pillar diameter $8\,a_B$; $L_F = 2a_B$; $\theta_F = 70°$ . The impact of algal rotation has been modelled by including a periodic rotation of the flagellar beads in the equations of motion.
